# Supplementary material for: Wasserstein Distances Made Explainable: Insights Into Dataset Shifts and Transport Phenomena
Source: arXiv:2505.06123 source file (2026-03-01)
Supplement: Supplementary file 1 [file supplement.pdf]

# Wasserstein Distances Made Explainable: Insights into Dataset Shifts and Transport Phenomena

(Supplementary Notes)

Philip Naumann Jacob Kauffmann Grégoire Montavon

This document contains supplementary notes that provide more details on the content of the main text "Wasserstein Distances Made Explainable: Insights into Dataset Shifts and Transport Phenomena". We provide additional proofs, derivations, figures, and experimental details to support the main text's conceptual, technical, and experimental parts.

## Supplementary Note A: Sensitivity of Explanations to the Wasserstein Model

In this note, we provide qualitative results showing how $\mathcal{W}$aX's attribution exhibits better sensitivity to the specification of the Wasserstein model than the actual transport map. Two examples are shown in Fig. 1. In the first example, we consider a transport phenomenon of an incompressible fluid moving from left to right and passing through a bottleneck. While different specifications of the Wasserstein distance lead to roughly the same transport solution, the key contributors to the Wasserstein distance change drastically, with the bottleneck playing an increasingly important role with large values of $p$. This increasingly important role is faithfully reflected in explanations produced by $\mathcal{W}$aX, whereas the data, its coupling, and derived explanations are largely insensitive. In the second example, building on a real dataset and attributing this time on input features, similar high sensitivity of our $\mathcal{W}$aX method compared to the coupling distribution is highlighted, with the most relevant features changing significantly whether we consider $\mathcal{W}_1$ or $\mathcal{W}_4$.

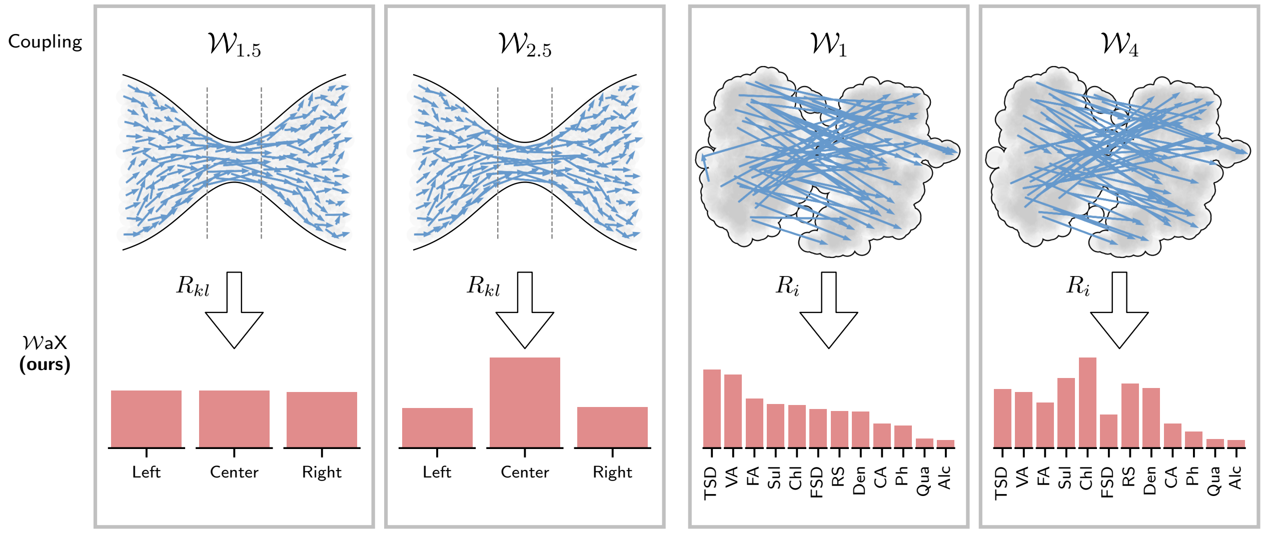


Figure 1: On the left, rightward shift of an incompressible fluid through a bottleneck by identifying the contributions of points (cf. Eq. (3a) from the main text) before, in, and after a bottleneck to the Wasserstein distance. On the right, $\mathcal{W}$aX identifies features that contribute to the shift between red and white wine in terms of input features (cf. Eq. (3b) from the main text). The arrows visualizing the coupling distribution are clustered (cf. [1]) for ease of visualization.

## Supplementary Note B: Proofs of Propositions 1 and 2

In this note, we provide the mathematical derivations supporting Propositions 1 and 2 from the main text. Specifically, we show how the relevance scores $R_{kl}$ and $R_i$ align with gradient-based computations under the choice of hyperparameters $\alpha = p$ and $\beta = q$, respectively.

**Proposition 1.** *When choosing $\alpha = p$, the relevance scores $R_{kl}$ of pairs of points can be expressed as the gradient computation $R_{kl} = (\partial \mathcal{W}_p / \partial z_{kl}) \cdot z_{kl}$, where we treat $\gamma^\star$ as a constant.*

*Proof.*

$$\begin{aligned} \frac{\partial \mathcal{W}_p}{\partial z_{kl}} \cdot z_{kl} &= \left( \frac{\partial}{\partial z_{kl}} \Big( \sum_{ij} \gamma^\star_{ij} \cdot z^p_{ij} \Big)^{1/p} \right) \cdot z_{kl} \\ &= \left( \Big( \sum_{ij} \gamma^\star_{ij} \cdot z^p_{ij} \Big)^{1/p-1} \cdot \gamma^\star_{kl} \cdot z^{p-1}_{kl} \right) \cdot z_{kl} \\ &= \frac{\gamma^\star_{kl} \cdot z^p_{kl}}{\sum_{kl} \gamma^\star_{kl} \cdot z^p_{kl}} \mathcal{W}_p \\ &= R_{kl} \end{aligned}$$

□

**Proposition 2.** *When choosing $\alpha = p$ and $\beta = q$, the relevance scores $R_i$ of the input features can be expressed as the gradient computation $R_i = (\partial \mathcal{W}_p / \partial x_{:,i})^\top x_{:,i} + (\partial \mathcal{W}_p / \partial y_{:,i})^\top y_{:,i}$, where $\gamma^\star$ is again treated as constant.*

*Proof.* First, note that for any pair $(x, y)$ and $0 < q < \infty$ we can expand as follows:

$$\begin{aligned} \frac{\partial \|x - y\|_q}{\partial x_i} \cdot x_i + \frac{\partial \|x - y\|_q}{\partial y_i} \cdot y_i &= (\textstyle\sum_i |x_i - y_i|^q)^{\frac{1}{q}-1} \cdot |x_i - y_i|^{q-1} \cdot (x_i \cdot \mathrm{sgn}(x_i - y_i) + y_i \cdot \mathrm{sgn}(y_i - x_i)) \\ &= \frac{|x_i - y_i|^q}{\sum_i |x_i - y_i|^q} \cdot \|x - y\|_q \end{aligned}$$

where sgn is the sign function. Next, we apply the chain rule and use Proposition 1 from the main text as an intermediate step:

$$\begin{aligned} \frac{\partial \mathcal{W}_p}{\partial x_{:,i}}^\top x_{:,i} + \frac{\partial \mathcal{W}_p}{\partial y_{:,i}}^\top y_{:,i} &= \sum_{kl} \frac{\partial \mathcal{W}_p}{\partial z_{kl}} \cdot \left( \frac{\partial z_{kl}}{\partial x_{k,i}} x_{k,i} + \frac{\partial z_{kl}}{\partial y_{l,i}} y_{l,i} \right) \\ &= \sum_{kl} \frac{R_{kl}}{z_{kl}} \cdot \left( \frac{|x_{k,i} - y_{l,i}|^q}{\sum_i |x_{k,i} - y_{l,i}|^q} \cdot z_{kl} \right) \\ &= \sum_{kl} \frac{|x_{k,i} - y_{l,i}|^q}{\sum_i |x_{k,i} - y_{l,i}|^q} \cdot R_{kl} \\ &= R_i \end{aligned}$$

□

## Supplementary Note C: Choosing $\mathcal{W}$aX Hyperparameters

This note empirically supports the choice of our proposed $\mathcal{W}$aX $\alpha, \beta$-hyperparameter heuristic as proposed in Section III from the main text:

$$\begin{aligned} \alpha &= p \\ \beta &= \min(p + 2, q) \end{aligned}$$

assuming $p \ll \infty$. We use the 'Mice' dataset [2] due to its high dimensionality. We iterate over different model parameters $p$ and $q$, and explanation parameters $\alpha$ and $\beta$ to study how they influence the SRG metric (Eq. (5) from the main text). We see in Fig. 2 that our heuristic for choosing $\alpha$ and $\beta$ (blue marker) is always within or close to the optimal parameter area in terms of SRG score (yellow), as visualized by the contour lines.

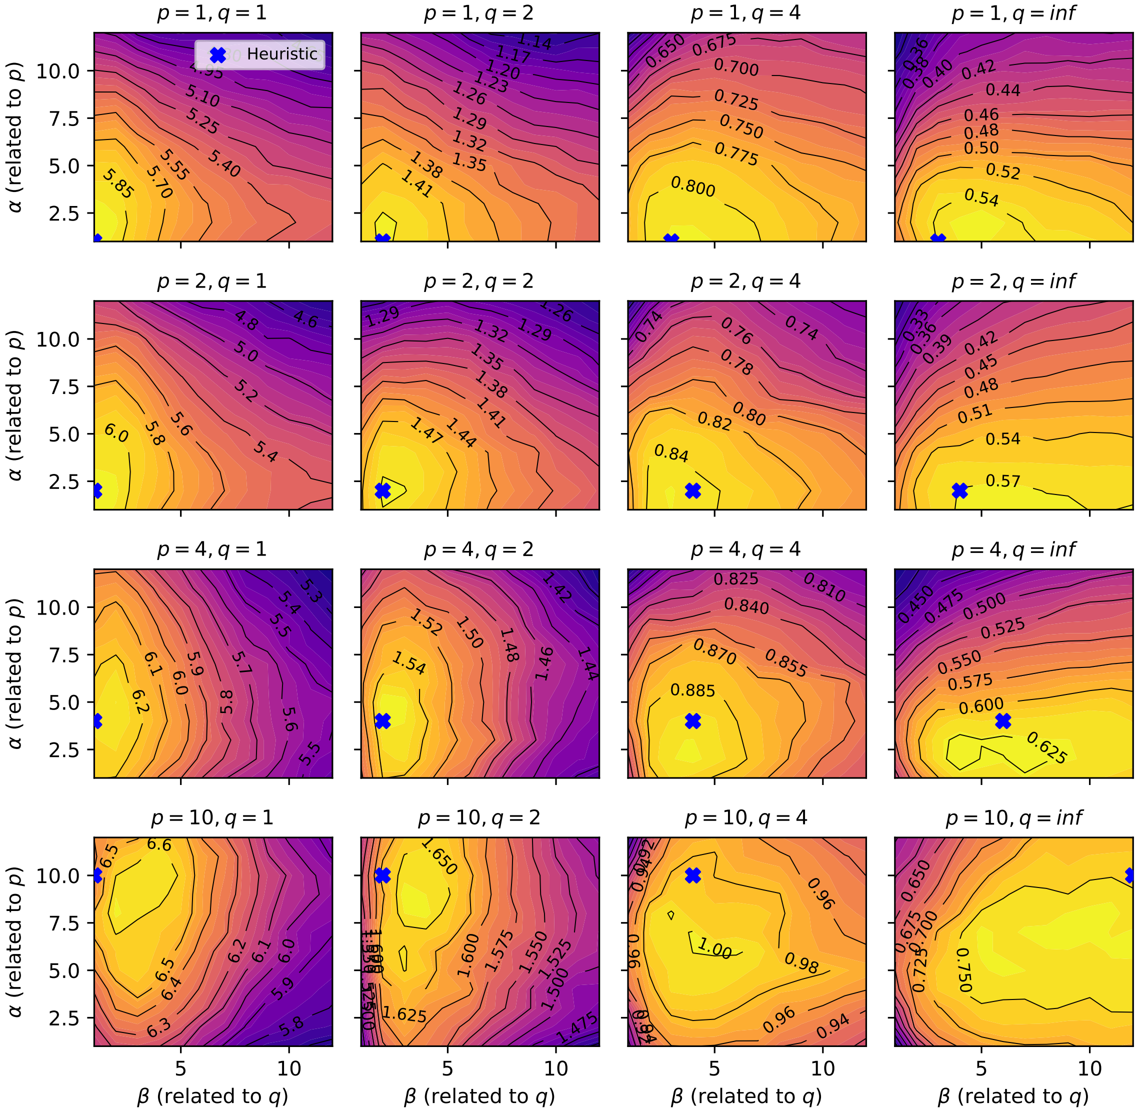


Figure 2: Effect of $\mathcal{W}$aX hyperparameters ($\alpha$ and $\beta$) on the SRG performance metric (Eq. (5) from the main text) for various specifications of the Wasserstein distance (parameters $p$ and $q$) and applied to the 'Mice' dataset. The highest SRG values are shown in yellow. Each plot shows our heuristic for choosing the hyperparameters $\alpha$ and $\beta$ as an annotated blue marker.

## Supplementary Note D: Datasets Used and Preprocessing

All tabular datasets used in Tables I and III and Section VI from the main text are taken from the "UCI machine learning repository" [3].

In *Section IV-A* from the main text, the tabular datasets were preprocessed by retaining only real-valued features, removing features and instances with a high proportion of missing values, eliminating duplicate instances, removing strong outliers where any feature value deviates more than three standard deviations from its mean, standardizing features to zero mean and unit variance, and imputing remaining missing values using nearest-neighbor imputation. In the case of the 'Crime' dataset [4], we only use the features considered in [13] as the starting point (hence the much lower number in Table I from the main text in comparison to the original dataset in Table 1).

In *Section IV-B* from the main text, the time series datasets are similarly preprocessed as in Section IV-A from the main text. We remove features with too many missing values and samples with any missing values, removing strong outliers where any feature value deviates more than three standard deviations from its mean, and standardizing to zero mean and unit variance. When a sample

| Section | Dataset | $N$ | $d$ | Missing Values | Ref. |
|---|---|---|---|---|---|
| IV-A | Crime | 1994 | 127 | ✓ | [4] |
| | Mice | 1080 | 80 | ✓ | [2] |
| | Musks1 | 476 | 168 | - | [5] |
| | Robot | 463 | 90 | - | [6] |
| | Wine | 4898 | 12 | - | [7] |
| | Wisconsin | 569 | 30 | - | [8] |
| IV-B | Air Quality | 9358 | 15 | ✓ | [9] |
| | Electricity | 2 075 259 | 9 | ✓ | [10] |
| | Appliances | 19 735 | 28 | - | [11] |
| VI | Abalone | 4177 | 8 | - | [12] |

Table 1: Tabular datasets used in the main text. The number of samples $N$ and dimensions $d$ refer to the *original* datasets. The values after preprocessing (e.g. removing categorical features, missing values, outliers, etc.) used in the experiments can be found in the main text tables.

is eliminated in this process, we also delete its corresponding coupled match to ensure that we always have ground-truth couplings.

In *Section VI* from the main text, we remove the categorical 'sex' feature from the Abalone dataset. Then, we standardize the remaining features to zero mean and unit variance. Finally, we remove strong outliers, i.e. those where any feature value deviates more than three standard deviations from its mean, to prevent them from spuriously influencing the subsequent analysis.

## Supplementary Note E: Experimental Details for Section IV-B

The evaluation is performed over three different time series datasets (see Table 1 in Supplementary Note D), with temporal shifts $\Delta t$ ranging from 1 to 6, and results are averaged over all source times $t \in \{0, \dots, 23\}$. Our $\mathcal{W}$aX method is applied with two Wasserstein distance models, the classical one (with coupling $\gamma^\star$) and a maximally regularized [14] one (with coupling $\gamma^\star_{\text{reg}} = \text{cst.}$).

We create subset splits $\widetilde{\mathcal{D}}_\mathcal{S} = \{(x_{t+kT})\}_{k\in\mathcal{K}_1}$ and $\widetilde{\mathcal{D}}_\mathcal{T} = \{(x_{t+\Delta t+kT})\}_{k\in\mathcal{K}_2}$ to avoid exposing the ground truth coupling. These are subsets of the original data $\mathcal{D}_\mathcal{S}$ and $\mathcal{D}_\mathcal{T}$, respectively, with $\mathcal{K}_1$ and $\mathcal{K}_2$ being disjoint, thus defining a random partition of $\mathbb{Z}$. This setup simulates a scenario where $\mathcal{W}$aX has access to the data distributions but not the exact same instances evolving from source to target. In our evaluation benchmark, we only use time delays less than or equal to six hours to guarantee reasonable mutual information between source and target. We only retain cases where at least 50 source and target instances are available for characterizing the transport.

For the experiments on the PLISM dataset [15], we also partition the data into random, non-overlapping subsets for the evaluated methods.

## Supplementary Note F: Attributing KL Divergence

In this note, we provide the mathematical details for attributing the Kullback-Leibler (KL) divergence, as discussed in Section IV-B from the main text.

We first consider the case where the source and target distributions are isotropic Gaussian (or modeled as such), specifically:

$$\mu(x) = \mathcal{N}(m, \sigma^2 I)$$
$$\nu(x) = \mathcal{N}(-m, \sigma^2 I)$$

We get the following expression for the KL divergence:

$$\begin{aligned} D_{\mathsf{KL}}(\mu \parallel \nu) &= \mathbb{E}_\mu\Big[\log\frac{\mu(x)}{\nu(x)}\Big] \\ &= \mathbb{E}_\mu\Big[-\frac{1}{2\sigma^2}\|x-m\|^2 + \frac{1}{2\sigma^2}\|x+m\|^2\Big] \\ &= \mathbb{E}_\mu\Big[2\frac{x^\top m}{\sigma^2}\Big] \\ &= \frac{2\|m\|^2}{\sigma^2} \end{aligned}$$

Likewise, we get

$$\begin{aligned} D_{\mathsf{KL}}(\nu \parallel \mu) &= \mathbb{E}_\nu\Big[\log\frac{\nu(x)}{\mu(x)}\Big] \\ &= \frac{2\|m\|^2}{\sigma^2} \end{aligned}$$

The symmetrized KL divergence can be attributed to the input features as:

$$\mathcal{E}\big\{D_{\mathsf{KL}}(\mu \parallel \nu) + D_{\mathsf{KL}}(\nu \parallel \mu)\big\}_i = 4\frac{m_i^2}{\sigma^2}$$

In other words, attribution is proportional to the square difference between the source and target means along each dimension and is also equivalent to attribution of a mean shift.

When classifying the data using a logistic classifier (including nonlinear versions of it), and assuming that source and target distributions are given the same weight during training, the output of the classifier $f(x)$ is interpretable as the log-density ratio $\log[\mu(x)/\nu(x)]$. This gives:

$$\begin{aligned} D_{\mathsf{KL}}(\mu \parallel \nu) &= \mathbb{E}_\mu\Big[\log\frac{\mu(x)}{\nu(x)}\Big] \\ &= \mathbb{E}_\mu[f(x)] \end{aligned}$$

and similarly

$$\begin{aligned} D_{\mathsf{KL}}(\nu \parallel \mu) &= \mathbb{E}_\nu\Big[\log\frac{\nu(x)}{\mu(x)}\Big] \\ &= \mathbb{E}_\nu[-f(x)] \end{aligned}$$

where $f$ is a model (e.g. a logistic classifier or a neural network). Attribution of the symmetrized KL-divergence thus proceeds as:

$$\mathcal{E}\big\{D_{\mathsf{KL}}(\mu \parallel \nu) + D_{\mathsf{KL}}(\nu \parallel \mu)\big\}_i = \mathbb{E}_\mu\big[\mathcal{E}\{f(x)\}_i\big] + \mathbb{E}_\nu\big[\mathcal{E}\{-f(x)\}_i\big]$$

The attribution of the classifier logit $f(x)$ can be carried out using existing attribution techniques such as LRP (cf. [16, 17]). When $f$ is a linear classifier, i.e. $f(x) = w^\top x + b$, GI becomes a mean shift weighted by $w$: $R_i = \mathbb{E}_\mu[w_i x_i] + \mathbb{E}_\nu[-w_i x_i] = w_i(\mathbb{E}_\mu[x_i] - \mathbb{E}_\nu[x_i]) = w_i(\bar{x}_i - \bar{y}_i)$, where $\bar{x}$ and $\bar{y}$ are source and target mean. Another attribution scheme uses the sensitivity of the function, i.e. $R_i = |\frac{\partial f}{\partial x_i}|^p = |w_i|^p$ with $p \geq 1$.

## Supplementary Note G: Closed Form Solution for $\boldsymbol{U}$-$\mathcal{W}$aX

This note provides a closed-form solution for $\boldsymbol{U}$-$\mathcal{W}$aX in the special case of $r = 2$ and $C = 1$. For this special case, the orthogonal matrix used for modeling subspaces in Section V from the main text reduces to a two-block matrix

$$\boldsymbol{U} = (U \,|\, U_\perp) \tag{1}$$

where $U$ is the subspace we would like to optimize and $U_\perp$ is the orthogonal complement. The $\boldsymbol{U}$-$\mathcal{W}$aX objective similarly reduces to a measure of the spread of shifts expressed in the given subspace:

$$Q = \Big( \sum_{kl} \gamma^\star_{kl} \cdot z^2_{kl} \Big)^{1/2} \tag{2}$$

$$\text{where} \quad z_{kl} = \|U^\top (x_k - y_l)\|_2 \tag{3}$$

It can then be shown that the optimization problem can be carried out in closed form:

$$\begin{aligned} \operatorname*{argmax}_{\boldsymbol{U}} \{Q\} &= \operatorname*{argmax}_{\boldsymbol{U}} \{Q^2\} \\ &= \operatorname*{argmax}_{\boldsymbol{U}} \Big\{ \sum_{kl} \gamma^\star_{kl} \cdot \|U^\top (x_k - y_l)\|_2^2 \Big\} \\ &= \operatorname*{argmax}_{\boldsymbol{U}} \big\{ \mathrm{Tr}(U^\top S U) \big\} \end{aligned}$$

subject to $\boldsymbol{U}^\top \boldsymbol{U} = I$, and where $S = \sum_{kl} \gamma^\star_{kl} (x_k - y_l)(x_k - y_l)^\top$. This is a canonical form similar to that of PCA, where the subspace $U$ spans the leading eigenvectors of the matrix $S$.

Interestingly, PCA can be seen as a special case of the problem above where the target instances are set to the mean source instances (i.e. $y_l = \bar{x}$). This special case can be interpreted as the subspace that maximally expresses the transport of source data points to their means or vice versa.

## References


[1] S. Kulinski and D. I. Inouye. Towards explaining distribution shifts. In *ICML*, volume 202 of *Proceedings of Machine Learning Research*, pages 17931–17952. PMLR, 2023.

[2] C. Higuera, K. J. Gardiner, and K. J. Cios. Mice protein expression. `https://doi.org/10.24432/C50S3Z`, August 2015.

[3] M. Kelly, R. Longjohn, and K. Nottingham. The UCI machine learning repository. `https://archive.ics.uci.edu`, 2023.

[4] M. Redmond. Communities and crime. `https://doi.org/10.24432/C53W3X`, July 2009.

[5] D. Chapman and A. N. Jain. Musk (version 1). `https://doi.org/10.24432/C5ZK5B`, September 1994.

[6] L. S. Lopes and L. M. Camarinha-Matos. Robot execution failures. `https://doi.org/10.24432/C5M89N`, April 1999.

[7] P. Cortez, A. Cerdeira, F. Almeida, T. Matos, and J. Reis. Wine quality. `https://doi.org/10.24432/C56S3T`, October 2009.

[8] W. H. Wolberg, O. L. Mangasarian, and W. N. Street. Breast cancer wisconsin (diagnostic). `https://doi.org/10.24432/C5DW2B`, October 1995.

[9] S. D. Vito. Air quality. `https://doi.org/10.24432/C59K5F`, March 2016.

[10] G. Hébrail and A. Berard. Individual household electric power consumption. `https://doi.org/10.24432/C58K54`, August 2012.

[11] L. Candanedo. Appliances energy prediction. `https://doi.org/10.24432/C5VC8G`, February 2017.

[12] W. Nash, T. Sellers, S. Talbot, A. Cawthorn, and W. Ford. Abalone. `https://doi.org/10.24432/C55C7W`, November 1995.

[13] J. Gardner, Z. Popovic, and L. Schmidt. Benchmarking distribution shift in tabular data with TableShift. In *Advances in Neural Information Processing Systems*, volume 36, pages 53385–53432. Curran Associates, Inc., 2023.

[14] M. Cuturi. Sinkhorn Distances: Lightspeed Computation of Optimal Transport. In *Advances in Neural Information Processing Systems*, volume 26, pages 2292–2300. Curran Associates, Inc., 2013.

[15] A. Filiot, N. Dop, O. Tchita, A. Riou, R. Dubois, T. Peeters, D. Valter, M. Scalbert, C. Saillard, G. Robin, and A. Olivier. Distilling foundation models for robust and efficient models in digital pathology, 2025.

[16] S. Bach, A. Binder, G. Montavon, F. Klauschen, K.-R. Müller, and W. Samek. On pixel-wise explanations for non-linear classifier decisions by layer-wise relevance propagation. *PLOS ONE*, 10(7):1–46, July 2015.

[17] G. Montavon, A. Binder, S. Lapuschkin, W. Samek, and K.-R. Müller. Layer-wise relevance propagation: An overview. In *Explainable AI*, volume 11700 of *Lecture Notes in Computer Science*, pages 193–209. Springer, 2019.
